# Supplementary material for: Testing Spacecraft Formation Flying with Crazyflie Drones as Satellite Surrogates
Source: arXiv:2402.14750 source file (2024-02-22)
Supplement: Supplementary file 1 [file Appendix_B_Technical_Details.tex]

\textcolor{red}{This is from the readme on gitlab and the information will be rewritten as an appendix} \\

This project uses linearized Clohessy-Wiltshire dynamics in Hill's frame to create relative spacecraft trajectories. These trajectories, implemented in both continuous and discrete representations, are created for a satellite with prescribed mass and mean motion, and then scaled and formatted for use as waypoints defining the desired trajectory of a crazyflie. This project uses the gym-pybullet-drones gym environment to simulate the flight of crazyflie 2.1 drones. The creation, scaling, and formatting of trajectories following from the CWH equations, their use in plotting and as a desired trajectory, and slight adjustment of PID gains is a major contribution of this project. This allows for the simulated testing of spacecraft dynamics using crazyflie drones as a satellite surrogate, and the simulated testing of reinforcement learning controlled satellite trajectories in this same gym environment is currently being developed.

List of Features:
- Trajectory made from full Linearized Clohessy-Wiltshire equations in Hill's frame - both natural motion trajectories and controlled trajectories can be tested
- Trajectory can be made in either discrete or continuous representation, and all features fully implemented into both
- All variables defined in single class and only ever need to be updated in one place:
  - Initial conditions can be changed, and trajectory, waypoints, and plotted trajectory are all updated simultaneously for both implementations making tests simple and intuitive to change
    - Same goes for satellite control vector u
  - Orbital period can be adjusted
  - Trajectory run time tied to simulation run time - if runtime is made longer, exact number of needed waypoints for simulated flight are saved without changing orbital period
  -  Coordinate system the trajectory is written in is a global x, y, z coordinate system nearly identical to the coordinate system used by the crazyflie lighthouse positioning system, meaning this code is already mathematically structured for physical testing

Any significant contribution is marked by authorship at the beginning of the respective file - if there is no authorship
at the beginning of a file, it is to be assumed to be authored by the team that made gym-pybullet-drones

%%% Showing Controlled Trajectories %%%

Figures \ref{fig:Controlled_Trajectory_3D} and \ref{fig:Controlled_Trajectory_2D} show how the trajectory is changed when control forces are introduced. The initial conditions are as follows:
\begin{equation}
    \centering
    \begin{matrix}
        x =  800 [m] & \dot{x} = 0.16 [m/s]\\
        \\
        y = \frac{2\dot{x}}{n} [m] & \dot{y} = -2nx [m/s]\\
        \\
        z = 1 & \dot{z} = 1\\
    \end{matrix}
    \label{eqn: ICs_out_of_plane}
\end{equation}
with control vector
\begin{equation}
    \centering
    \begin{matrix}
        u_x  = 0.005 [N]\\
        \\
        u_y  = 0.005 [N]\\
        \\
        u_z  = 0.005 [N]\\
    \end{matrix}
    \label{eqn: ICs}
\end{equation}

\begin{figure}[htb!]
    \centering
    \includegraphics[width = .49\textwidth]{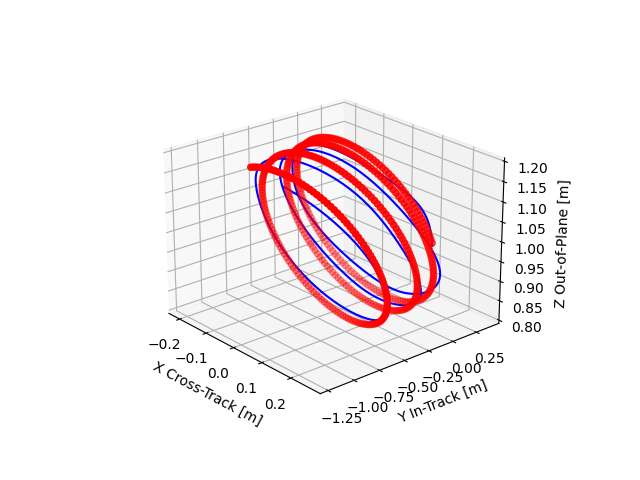}
    \caption{3D Plot of Out of Plane Controlled Waypoint Tracking with Tuned PID}
    \label{fig:Controlled_Trajectory_3D}
\end{figure}

\begin{figure}[htb!]
    \centering
    \includegraphics[width = .49\textwidth]{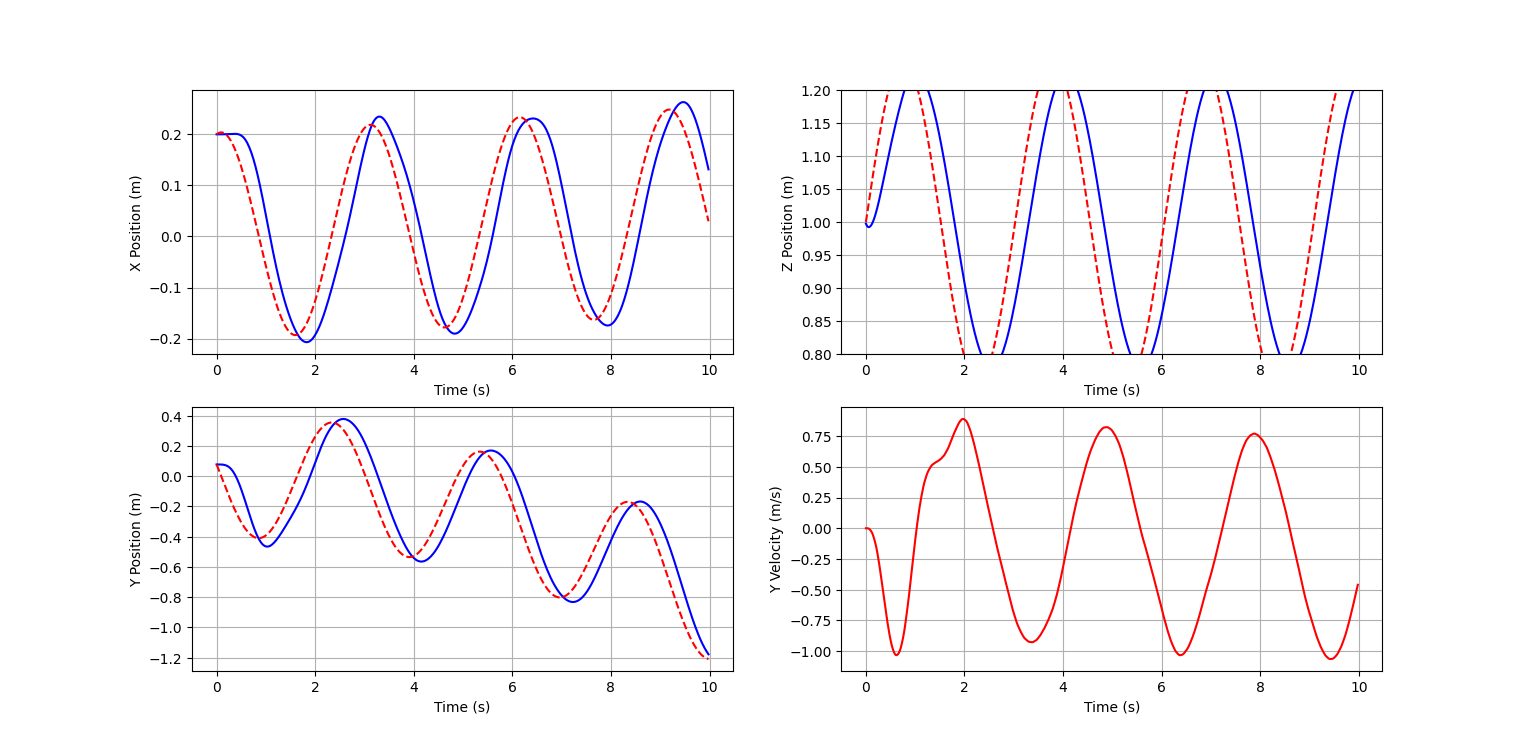}
    \caption{2D Plots of Out of Plane Controlled Waypoint Tracking with Tuned PID}
    \label{fig:Controlled_Trajectory_2D}
\end{figure}
