# Supplementary material for: Testing Spacecraft Formation Flying with Crazyflie Drones as Satellite Surrogates
Source: arXiv:2402.14750 source file (2024-02-22)
Supplement: Supplementary file 2 [file Appendix_A_CF_Platform.tex]

\subsection{Crazyflie Documentation}
This section is meant to detail information about the crazyflie and related bitcraze products relevant to this project. 
\textcolor{red}{Potential subsections - coordinate system, discussion of sim2real(coords, coding language, positioning system, flight controller, communication/control frequency, ...)}

\subsection{Crazyflie 2.1 Micro-quadcopter}
The Bitcraze Crazyflie 2.1 micro-quadcopter is an open source 6-degree of freedom quad-rotor drone platform designed with research applications in mind. It is small, inexpensive, and supports expansion decks that allow for additional capabilities such as the use of a positioning system, wireless charging, data logging, distance/motion sensors, and so forth. 
\begin{figure}[htb!]
    \centering
    \includegraphics[width = .30\textwidth]{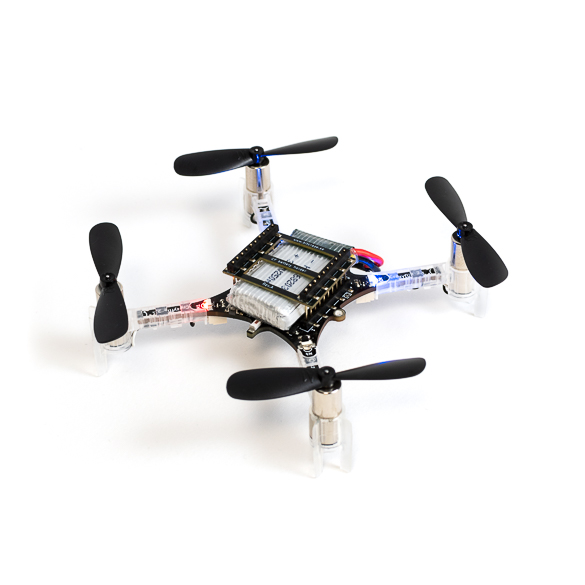}
    \caption{Bitcraze Crazyflie 2.1. \cite{CrazyfliePic}}
    \label{fig:BitcrazeCrazyflie21}
\end{figure}

\subsection{Lighthouse Positioning System}

\subsection{Relevant Specifications}
